# Supplementary material for: Monolayer Spontaneous Curvature of Raft-Forming Membrane Lipids
Source: arXiv:1307.0367 source file (2013-09-17)
Supplement: Supplementary file 1 [file supplementary.pdf]

# Supplementary Material for: Monolayer Spontaneous Curvature of Raft-Forming Membrane Lipids

Benjamin Kollmitzer, Peter Heftberger, Michael Rappolt, and Georg Pabst

September 17, 2013, Graz

## S1 Electron density calculation

All recognizable peaks of the intensity $I(q)$ were individually fitted using least-squares plus a linear background estimator, yielding peak intensities $I_{h,k}$ and positions $q_{h,k}$. The (1,1) and (2,0) peaks are close and were fitted together with a common linear background (Fig. S1).

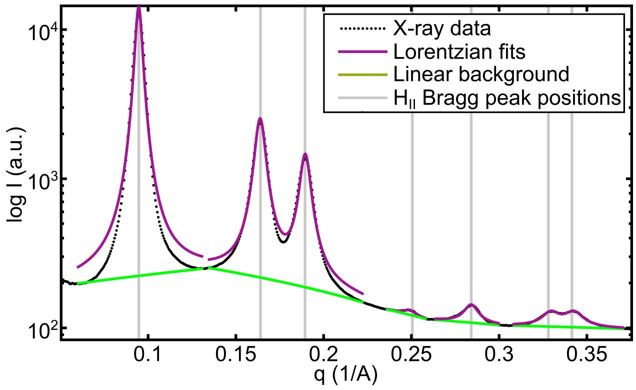


Figure S1: Analysis of DOPE at 35 °C.

We followed the procedure described by Rappolt *et al.*[1] for calculating electron maps. The lattice parameter $a$ was determined via the reflection law $\sqrt{3}\,a\,q_{h,k}\,/\,4\pi = 1, \sqrt{3}, 2, \sqrt{7}, \ldots$. Fourier synthesis yielded the electron density in real-space

$$\rho(\vec{r}) = \sum_{h,k} \alpha_{h,k} \sqrt{\frac{I_{h,k}\, q_{h,k}^2}{m_{h,k}}} . \cos\left(2\pi\, \vec{q}_{h,k} \cdot \vec{r}\right), \tag{S1}$$

where multiplication of the intensity with $q_{h,k}^2$ is known as Lorentz correction[2], $m_{h,k}$ is the multiplicity of the equivalent diffraction planes (6 for $(1,0),(1,1),(3,0)\ldots$; 12 for $(2,1),(3,1),(3,2)\ldots$)

and $\alpha_{h,k}$ is the phase ($\pm 1$ for centrosymmetric structures as in this work). Literature[3–5] suggests $(+--++++++-)$ as phasing condition for DOPE-rich, fully hydrated $H_{II}$ phases. Figure S2 gives an example for a calculated electron density map. Other phase combinations were tested, but yielded electron densities incompatible with the known structure.

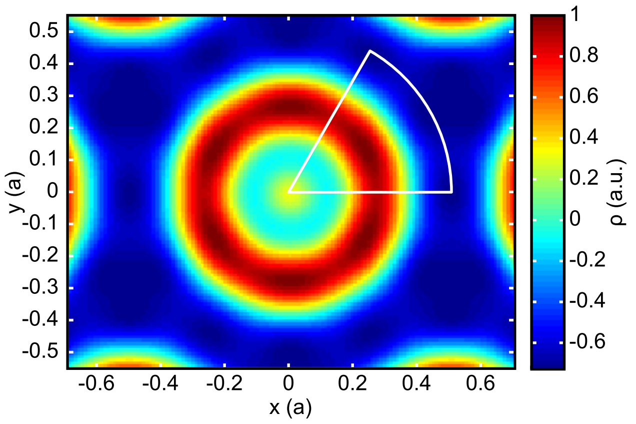


Figure S2: 2D electron density map $\rho(x,y)$ for DOPE at 35 °C. The white circular segment indicates the region, where the radial cross sections of $\rho$ are evaluated for the location of the pivotal plane. Coordinates are normalized by the unit cell parameter $a$.

A Gaussian fit to the radial cross section of the electron density yielded position $R_p$ and width $\sigma_p$ of the headgroup (Fig. S3). We averaged these quantities over azimuthal angles ranging from 0° ($x$-axis) to 60°, as indicated by the circular segment in Fig. S2.

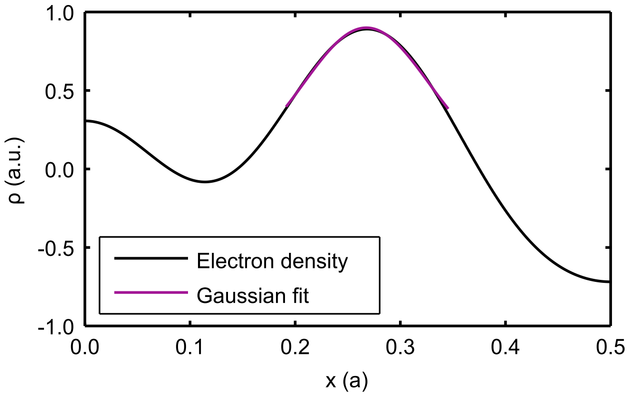


Figure S3: Radial cross section of the electron density from Fig. S2 along the $x$-axis with Gaussian fit for the headgroup region.

## S2 Tieline parameterization

For parameterizing coexistence regions and tieline fields, we applied the method described in[6,7]. Ternary phase diagram coordinates $(x,y,z)$ with $x+y+z=1$ and $\{x,y,z\}\in[0,1]$ are transformed into a two-dimensional vector $\vec{\Psi}=(\xi,\eta)$ with components $\xi=z\sqrt{3}/2$ and $\eta=y+z/2$. Bézier curves

$$\vec{B}(t)=\sum_{l=0}^{n}\binom{n}{l}(1-t)^{n-l}t^{l}\vec{P}_{l} \tag{S2}$$

of degree $n=5$ were reported to describe phase boundaries well in the $(\xi,\eta)$-space. To relate these curves to the tieline fields, Smith and coworkers[6] introduced the relationships

$$t_{Lo}(u)=\tau_c+(1-\tau_c)\,u \tag{S3}$$

$$t_{Ld}(u)=\tau_c-\frac{\tau_c\,u}{u+c\,(1-u)}, \tag{S4}$$

where $\tau_c$ characterizes the critical point and $c$ takes care of tieline fanning. Equations (S3) and (S4) allow to express the tieline endpoint compositions in 2D as $\vec{\Psi}_{Lo}(u)=\vec{B}(t_{Lo}(u))$ and $\vec{\Psi}_{Ld}(u)=\vec{B}(t_{Ld}(u))$, where $\vec{\Psi}_{Lo}(0)=\vec{\Psi}_{Ld}(0)$ describes the critical point.

We determined the 6 control points $\{\vec{P}_l\}$ from a least squares fit of the Bézier curves to the boundary coordinates of previously published compositional phase diagrams[7–9]. The fitting was performed with the MATLAB® function `grad7.m` listed in[10]. Having determined the control points, we calculated $\tau_c$, by minimizing the distance from the critical point to $\vec{B}(\tau_c)$. Analogously, the auxiliary points $\{\tau_{Lo,i},\tau_{Ld,i}\}$ were computed by minimizing the distance from $\vec{B}(\tau_{Lo/d,i})$ to the intersection of the $i$-th tieline with the phase boundary on the $L_o/L_d$ side. The parameter $c$ describing the tieline fanning was calculated by solving

$$c=\frac{(\tau_{Lo,i}-\tau_c)\;\tau_{Ld,i}}{(\tau_{Ld,i}-\tau_c)\;(\tau_{Lo,i}-1)} \tag{S5}$$

in the least squares sense. Equation (S5) follows directly from eliminating $u$ in Eqs. (S3) and (S4). The resulting parameters describing the reported tielines from[7–9] are listed in Tab. S1.

## S3 Line tension calculations

Based on elastic deformations of monolayers, Kuzmin *et al.*[11] derived an expression for the line tension $\gamma$ between two coexisting phases $L_o$ and $L_d$

$$\gamma=\frac{1}{Z}\sqrt{B_dK_dB_oK_o\frac{\delta^2}{h_0^2}}-\frac{1}{2Z}\left(J_{0,d}B_d-J_{0,o}B_o\right)^2, \tag{S6}$$

with $Z=\sqrt{B_dK_d}+\sqrt{B_oK_o}$, monolayer bending moduli $B$, tilt moduli $K$, monolayer spontaneous curvatures $J_0$, and structural parameters $\delta=h_o-h_d$ and $h_0=(h_o+h_d)/2$ relating the positions $h$ of the monolayer neutral planes. We refer to the first term of Eq. (S6) as elastic $\gamma_{el}$ and to the second as curvature contribution $\gamma_{J0}$ to the line tension. It was already pointed out in 4.2, that

Table S1: Parameters describing the tieline fields of published phase diagrams.

| | DOPC/DPPC/Chol§ | POPC/eggSM/Chol¶ | DOPC/DSPC/Chol‖ |
|---|---|---|---|
| $\vec{P}_0$ | (0.268, 0.568) | (0.438, 0.087) | (0.155, 0.074) |
| $\vec{P}_1$ | (0.204, 0.174) | (0.112, 0.029) | (0.176, 0.265) |
| $\vec{P}_2$ | (0.361, 0.252) | (0.531, 0.510) | (0.300, 0.380) |
| $\vec{P}_3$ | (0.603, 0.554) | (0.468, 0.126) | (0.624, 0.365) |
| $\vec{P}_4$ | (0.778, 0.196) | (0.671, 0.320) | (0.646, 0.391) |
| $\vec{P}_5$ | (0.780, 0.189) | (0.718, 0.208) | (0.764, 0.224) |
| $\tau_c$ | 0.429 | 0.297 | 0.506 |
| $c$ | 1.115 | 0.832 | 1.000 |

§ Phase diagram from[8]

¶ Phase diagram from[9]

‖ Values taken from[7], fits yielded similar results

these relations hold for $|J_0|$ much smaller than $1/h$. In the following examples, we therefore verify that $|J_0| \cdot h < 1$.

We calculate the spontaneous curvatures $J_{0,d}$ and $J_{0,o}$ according to Eq. (4) using known compositions of $L_o$ and $L_d$. The moduli in Eq. (S6) are effective moduli of the domains and normalized by cross-sectional area. Per-lipid tilt moduli $\kappa_j$ reported in[14] were taken, normalized by the lipid areas and averaged over the corresponding phase. Averaging was achieved by defining for each phase an average lipid, of volume $\bar{V} = \sum_j \chi_j V_j$ and area $\bar{A} = \bar{V}/h$, where $V_j$ is the volume of constituent lipid $j$ and $h$ the monolayer thickness of a given domain. We further assumed that the effective tilt modulus can be expressed as $K = \sum_j \chi_j \kappa_j / \bar{A}$.

Lipid volumes needed in this section are available in the literature:[12,13]

| | DOPC | POPC | DPPC | DSPC | Chol |
|---|---|---|---|---|---|
| $V$ ($nm^3$) | 1.30 | 1.26 | 1.23 | 1.35 | 0.63 |

## Example 1: Ternary mixtures

All parameters used for calculations are listed in Tab. S2. The magnitude of the spontaneous curvature $J_0$ is at least by a factor of 2 smaller than the monolayer thickness, meaning that the use of Eq. (S6) is justified. The resulting line tensions obtained by Eq. (S6) are reported in Tab. S3.

## Example 2: Varying domain sizes

For the quaternary mixture DOPC/POPC/DSPC/Chol, a similar calculation has already been used to rationalize the domain size behavior as a function of $\rho = \chi_{DOPC}/(\chi_{DOPC} + \chi_{POPC})$.[15] It was found, that the nanoscopic domains in POPC/DSPC/Chol grew bigger by replacing POPC with DOPC, until finally microscopic domains for DOPC/DSPC/Chol were detected. We repeat

Table S2: Compositions $\chi$, temperatures $T$, and elastic and structural parameters for Example 1.

| | DOPC/DPPC/Chol | | DOPC/DSPC/Chol | |
|---|---|---|---|---|
| | $L_d$ | $L_o$ | $L_d$ | $L_o$ |
| $\chi_1 : \chi_2 : \chi_3$ | 0.66:0.19:0.15 | 0.12:0.58:0.30 | 0.74:0.09:0.17 | 0.12:0.56:0.32 |
| $T$ (°C) | 15 | 15 | 22 | 22 |
| $B$ (kT) * | 17±2 | 49±3 | 15±1 | 53±4 |
| $\kappa_1$ (kT) * | 11±1 | 34±3 | 9±1 | 44±3 |
| $\kappa_2$ (kT) * | 14±1 | 53±3 | 10±1 | 60±4 |
| $\kappa_3$ (kT) * | 15±1 | 48±3 | 15±2 | 49±2 |
| $h$ (nm) *,† | 1.5 | 1.8 | 1.5 | 2.0 |
| $\bar{V}$ (nm$^3$) | 1.2 | 1.1 | 1.2 | 1.1 |
| $\bar{A}$ (nm$^2$) | 0.77 | 0.58 | 0.80 | 0.57 |
| $K$ (kT nm$^{-2}$) | 15 | 85 | 13 | 97 |
| $J_0$ (nm$^{-1}$) | -0.08 | -0.05 | -0.14 | -0.21 |
| $\|J_0\| \cdot h$ | 0.13 | 0.22 | 0.10 | 0.42 |

* Taken from [14]

† Although the thickness was not reported explicitly, it was used in the SAXS evaluation of [14]

Table S3: Resulting line tensions $\gamma$, and elastic $\gamma_{el}$ and curvature contributions $\gamma_{J0}$ for Example 1.

| | DOPC/DPPC/Chol | DOPC/DSPC/Chol |
|---|---|---|
| $\gamma_{el}$ (pN) | 1.4 | 3.4 |
| $\gamma_{J0}$ (pN) | 0.0 | -1.8 |
| $\gamma$ (pN) | 1.4 | 1.6 |

Table S4: Bilayer thickness $t$ and spontaneous curvature $J_0$ for Example 2.

| $\rho$ (%) | 0 | 5 | 10 | 17 | 20 | 35 | 100 |
|---|---|---|---|---|---|---|---|
| $t_{Ld}$ (nm) ‡ | 3.84 | 3.80 | 3.80 | 3.76 | 3.77 | 3.67 | 3.51 |
| $t_{Lo}$ (nm) ‡ | 4.48 | 4.48 | 4.48 | 4.46 | 4.46 | 4.46 | 4.48 |
| $J_{0,Ld}$ (nm$^{-1}$) | -0.06 | -0.06 | -0.06 | -0.07 | -0.07 | -0.08 | -0.12 |
| $J_{0,Lo}$ (nm$^{-1}$) | -0.16 | -0.16 | -0.17 | -0.17 | -0.17 | -0.18 | -0.19 |
| $\lvert J_{0,Ld}\rvert \cdot h_{Ld}$ | 0.09 | 0.10 | 0.10 | 0.11 | 0.11 | 0.12 | 0.18 |
| $\lvert J_{0,Lo}\rvert \cdot h_{Lo}$ | 0.30 | 0.31 | 0.32 | 0.32 | 0.33 | 0.34 | 0.38 |

‡ Taken from [15]

Table S5: Domain radii $R$ and resulting line tensions $\gamma$ with elastic $\gamma_{el}$ and curvature contributions $\gamma_{J0}$ for Example 2.

| $\rho$ (%) | 0 | 5 | 10 | 17 | 20 | 35 | 100 |
|---|---|---|---|---|---|---|---|
| $R$ (nm) ‡ | 68 | 85 | 98 | 111 | 124 | 162 | >225 |
| $\gamma_{el}$ (pN) | 1.7 | 1.9 | 1.9 | 2.1 | 2.0 | 2.7 | 4.1 |
| $\gamma_{J0}$ (pN) | -0.6 | -0.6 | -0.6 | -0.6 | -0.6 | -0.7 | -0.7 |
| $\gamma$ (pN) | 1.1 | 1.4 | 1.3 | 1.4 | 1.4 | 2 | 3.4 |

‡ Taken from [15]

that calculation, but with better determined values for bending moduli, tilt moduli and spontaneous curvature.

The compositions for DOPC/DSPC/Chol from Example 1 are similar to the compositions for $\rho = 1$. We use therefore these MD results[14] also for the current example. We further assume the per-lipid tilt moduli of POPC and DOPC to be equal. This means, that the results for $\rho = 1$ should be reliable, but become more imprecise with increasing POPC content. Bilayer thickness $t$ informations are taken from[15]. To obtain the height of the neutral plane $h$, which should be close to the apolar/polar interface[16], we subtract 0.3 nm from the monolayer thickness. This value is a reasonable guess for the distance between the Luzzatti position and the apolar/polar interface.[12] The applied bilayer thicknesses and monolayer spontaneous curvatures are listed in Tab. S4. Equation (S6) yields with these values the line tensions given in Tab. S5. Results are shown in Fig. 6. The magnitude of the spontaneous curvature $J_0$ is at least by a factor of 2 smaller than the monolayer thickness, meaning that the use of Eq. (S6) is justified.

## S4 Spontaneous curvature extrapolation

The dependence of $J_0^{mix}(T,\chi)$ on temperature $T$ and concentration $\chi$ is given in Tabs. S6–S12 and plotted in Figs. S4–S10. In the figures, black crosses depict valid data points used for extrapolation, while green data points were not considered because there $\chi > \chi_{crit}$.

Table S6: Spontaneous curvature $J_0^{mix}$ as function of temperature $T$ [°C] and concentration $\chi$ [mol%] Chol in DOPE. Numbers above $\chi_{crit}$ are untrustworthy

| | 10 mol% | 20 mol% | 30 mol% | 40 mol% | 50 mol% | $\chi_{crit}(mol\%)$ |
|---|---|---|---|---|---|---|
| 15 °C | −0.38 | −0.39 | −0.39 | −0.39 | −0.39 | > 40 |
| 25 °C | −0.40 | −0.40 | −0.41 | −0.41 | −0.41 | > 40 |
| 35 °C | −0.41 | −0.42 | −0.43 | −0.44 | −0.45 | > 40 |
| 45 °C | −0.43 | −0.44 | −0.45 | −0.46 | −0.47 | > 40 |
| 55 °C | −0.44 | −0.45 | −0.46 | −0.48 | −0.50 | > 50 |

Table S7: Spontaneous curvature $J_0^{mix}$ as function of temperature $T$ [°C] and concentration $\chi$ [mol%] DOPC in DOPE. Numbers above $\chi_{crit}$ and NaN are untrustworthy

| | 10 mol% | 20 mol% | 30 mol% | 40 mol% | 50 mol% | $\chi_{crit}(mol\%)$ |
|---|---|---|---|---|---|---|
| 15 °C | −0.34 | −0.30 | NaN | −0.24 | −0.22 | > 50 |
| 25 °C | −0.35 | −0.31 | NaN | −0.26 | −0.23 | > 50 |
| 35 °C | −0.36 | −0.33 | NaN | −0.27 | −0.25 | > 50 |
| 45 °C | −0.38 | −0.34 | NaN | −0.29 | −0.26 | > 50 |
| 55 °C | −0.39 | −0.36 | NaN | −0.30 | −0.27 | > 50 |

Table S8: Spontaneous curvature $J_0^{mix}$ as function of temperature $T$ [°C] and concentration $\chi$ [mol%] DPPC in DOPE. Numbers above $\chi_{crit}$ are untrustworthy

| | 10 mol% | 20 mol% | 30 mol% | 40 mol% | 50 mol% | $\chi_{crit}(mol\%)$ |
|---|---|---|---|---|---|---|
| 15 °C | −0.32 | −0.30 | −0.31 | −0.31 | −0.33 | > 10 |
| 25 °C | −0.33 | −0.29 | −0.26 | −0.25 | −0.28 | > 20 |
| 35 °C | −0.35 | −0.31 | −0.27 | −0.24 | −0.41 | > 20 |
| 45 °C | −0.37 | −0.32 | −0.28 | −0.25 | −0.24 | > 30 |
| 55 °C | −0.39 | −0.34 | −0.30 | −0.28 | −0.25 | > 30 |

Table S9: Spontaneous curvature $J_0^{mix}$ as function of temperature $T$ [°C] and concentration $\chi$ [mol%] DSPC in DOPE. Numbers above $\chi_{crit}$ and NaN are untrustworthy

| | 10 mol% | 20 mol% | 30 mol% | 40 mol% | 50 mol% | $\chi_{crit}(mol\%)$ |
|---|---|---|---|---|---|---|
| 15 °C | −0.35 | −0.35 | −0.35 | −0.35 | NaN | > 10 |
| 25 °C | −0.35 | −0.34 | −0.35 | −0.36 | NaN | > 10 |
| 35 °C | −0.36 | −0.34 | −0.34 | NaN | NaN | > 20 |
| 45 °C | −0.37 | −0.35 | −0.35 | −0.37 | NaN | > 20 |
| 55 °C | −0.39 | −0.36 | −0.34 | −0.34 | −0.27 | > 20 |

Table S10: Spontaneous curvature $J_0^{mix}$ as function of temperature $T$ [°C] and concentration $\chi$ [mol%] POPC in DOPE. Numbers above $\chi_{crit}$ and NaN are untrustworthy

| | 10 mol% | 20 mol% | 30 mol% | 40 mol% | 50 mol% | $\chi_{crit}(mol\%)$ |
|---|---|---|---|---|---|---|
| 15 °C | −0.33 | −0.29 | −0.25 | −0.22 | NaN | $> 40$ |
| 25 °C | −0.34 | −0.31 | −0.26 | −0.24 | NaN | $> 40$ |
| 35 °C | −0.36 | −0.32 | −0.28 | −0.25 | −0.22 | $> 40$ |
| 45 °C | −0.37 | −0.33 | −0.29 | −0.27 | −0.23 | $> 50$ |
| 55 °C | −0.38 | −0.34 | −0.30 | −0.27 | −0.24 | $> 50$ |

Table S11: Spontaneous curvature $J_0^{mix}$ as function of temperature $T$ [°C] and concentration $\chi$ [mol%] SOPC in DOPE. Numbers above $\chi_{crit}$ and NaN are untrustworthy

| | 10 mol% | 20 mol% | 30 mol% | 40 mol% | 50 mol% | $\chi_{crit}(mol\%)$ |
|---|---|---|---|---|---|---|
| 15 °C | −0.32 | −0.28 | −0.25 | −0.22 | −0.19 | $> 30$ |
| 25 °C | −0.34 | −0.30 | −0.27 | −0.23 | NaN | $> 30$ |
| 35 °C | −0.35 | −0.31 | −0.28 | −0.25 | −0.22 | $> 30$ |
| 45 °C | −0.37 | −0.33 | −0.30 | −0.27 | −0.22 | $> 30$ |
| 55 °C | −0.39 | −0.34 | −0.31 | −0.28 | −0.24 | $> 30$ |

Table S12: Spontaneous curvature $J_0^{mix}$ as function of temperature $T$ [°C] and concentration $\chi$ [mol%] eggSM in DOPE. Numbers above $\chi_{crit}$ and NaN are untrustworthy

| | 10 mol% | 20 mol% | 30 mol% | 40 mol% | 50 mol% | $\chi_{crit}(mol\%)$ |
|---|---|---|---|---|---|---|
| 15 °C | −0.35 | −0.28 | −0.29 | NaN | NaN | $> 10$ |
| 25 °C | −0.37 | −0.35 | −0.28 | NaN | NaN | $> 10$ |
| 35 °C | −0.38 | −0.36 | −0.30 | NaN | NaN | $> 10$ |
| 45 °C | −0.39 | −0.38 | −0.30 | NaN | NaN | $> 10$ |
| 55 °C | −0.39 | −0.39 | −0.33 | NaN | NaN | $> 10$ |

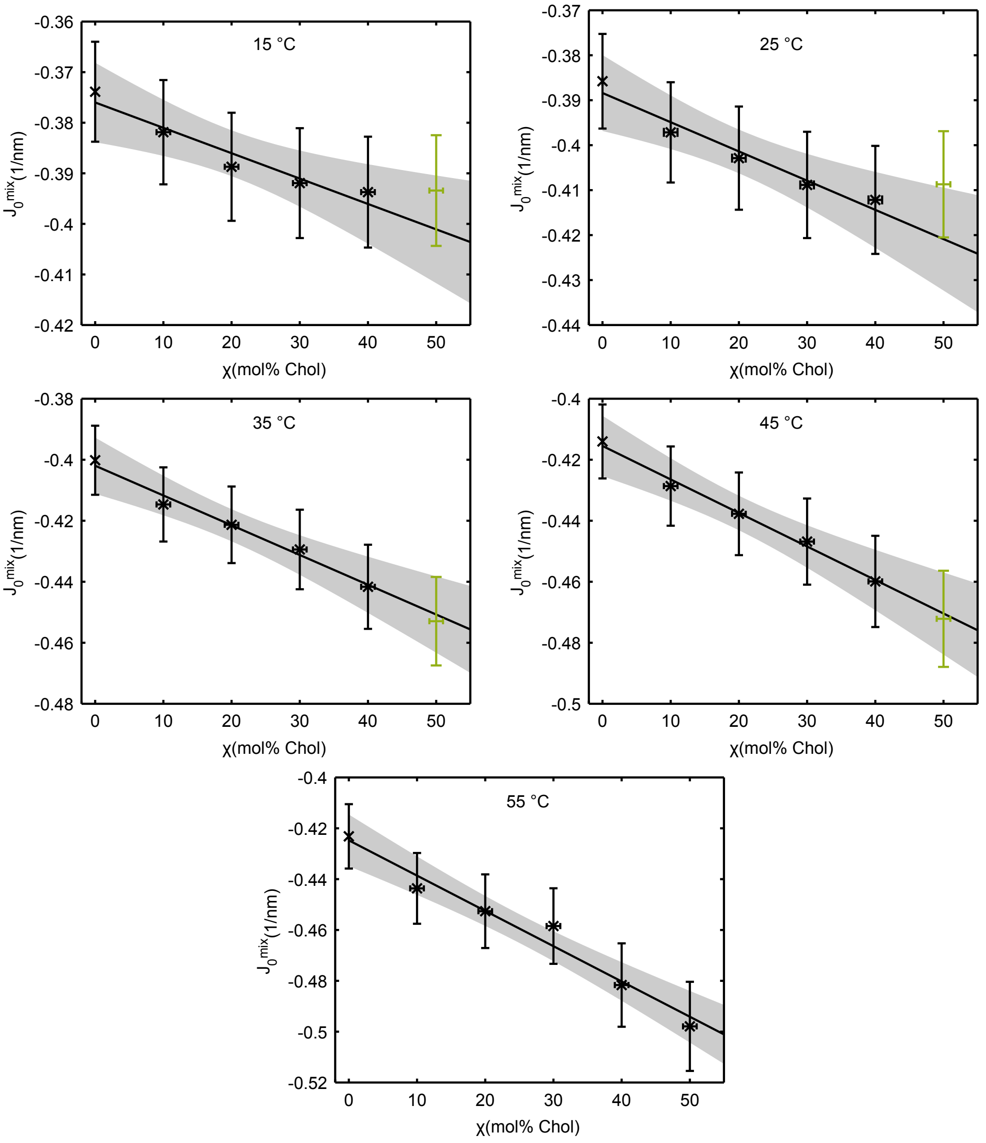


Figure S4: Determination of $J_0$ for Chol.

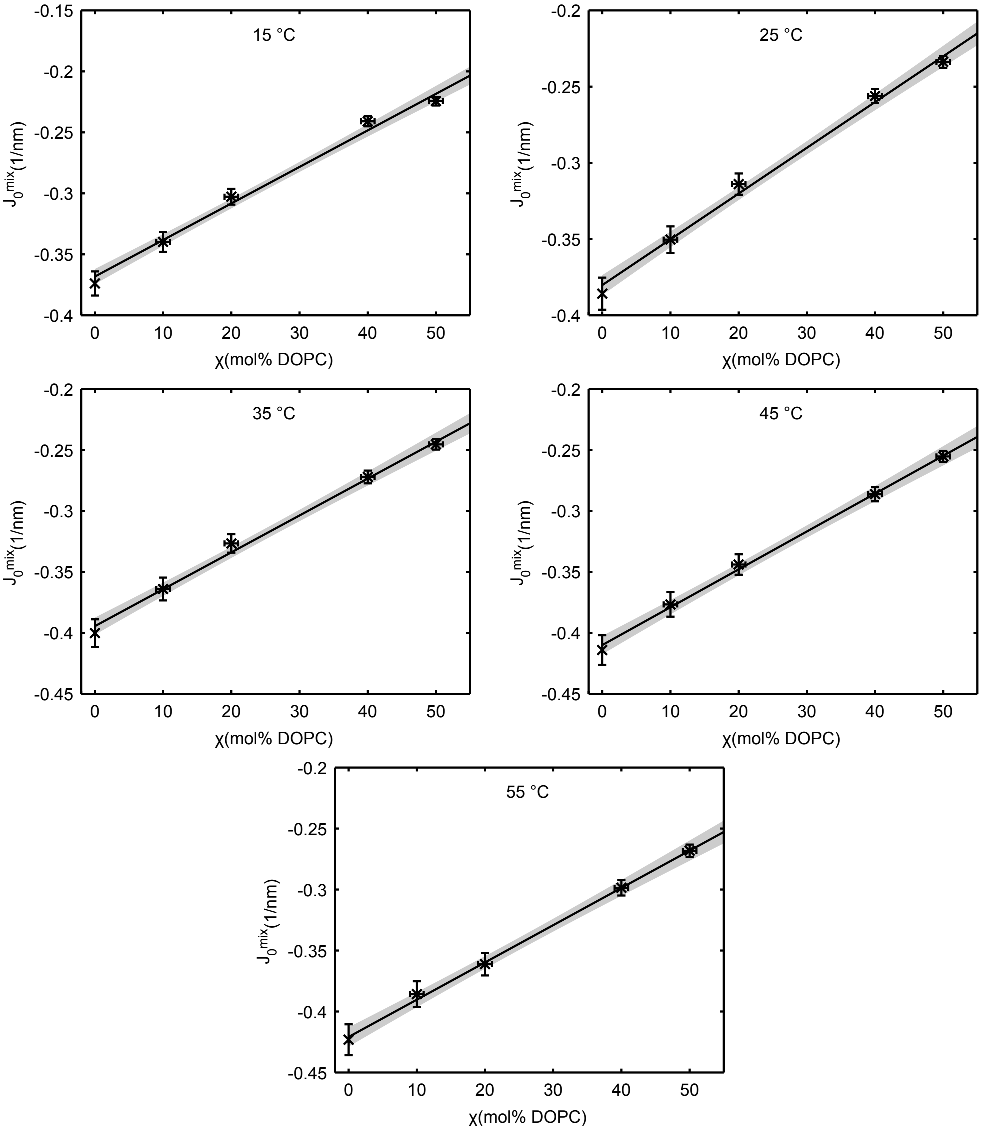


Figure S5: Determination of $J_0$ for DOPC.

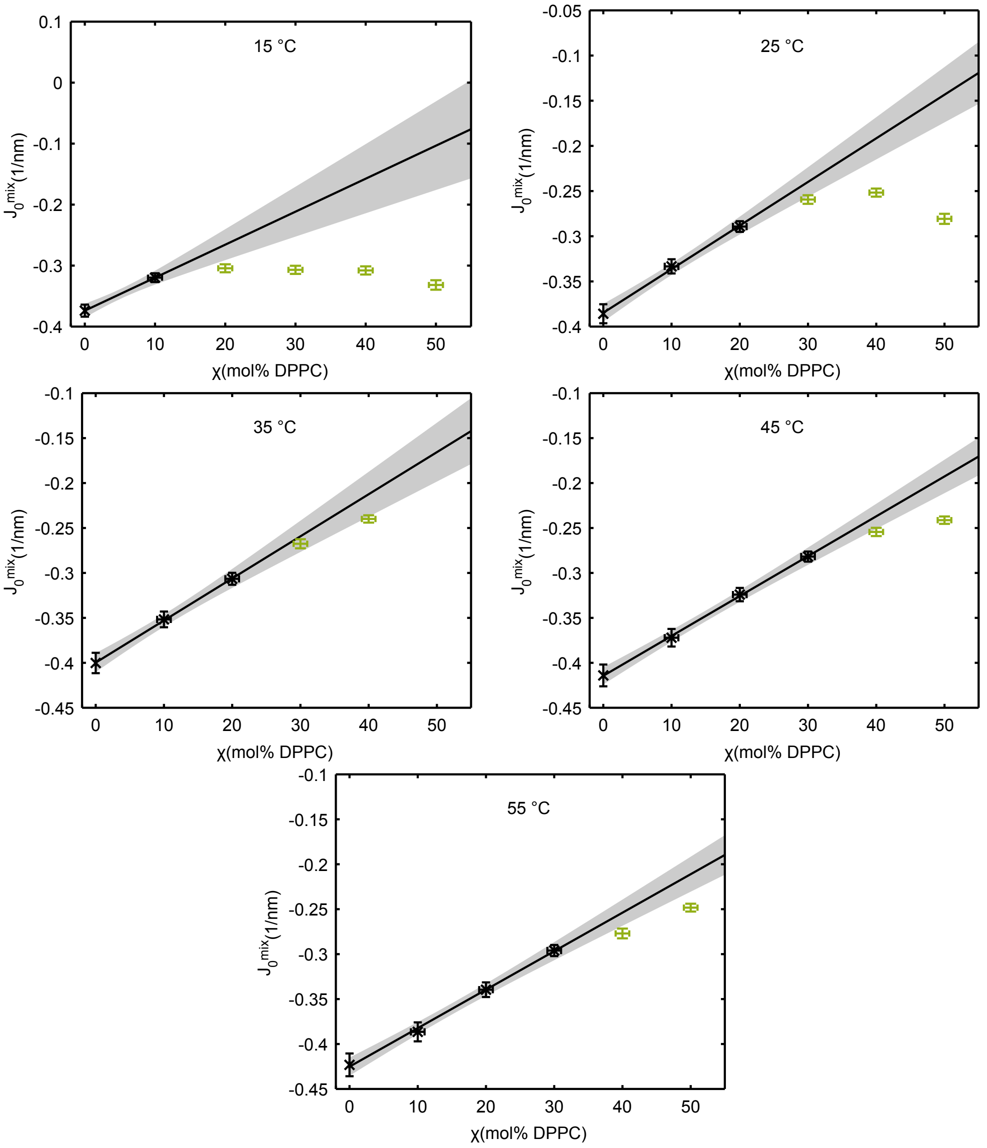


Figure S6: Determination of $J_0$ for DPPC.

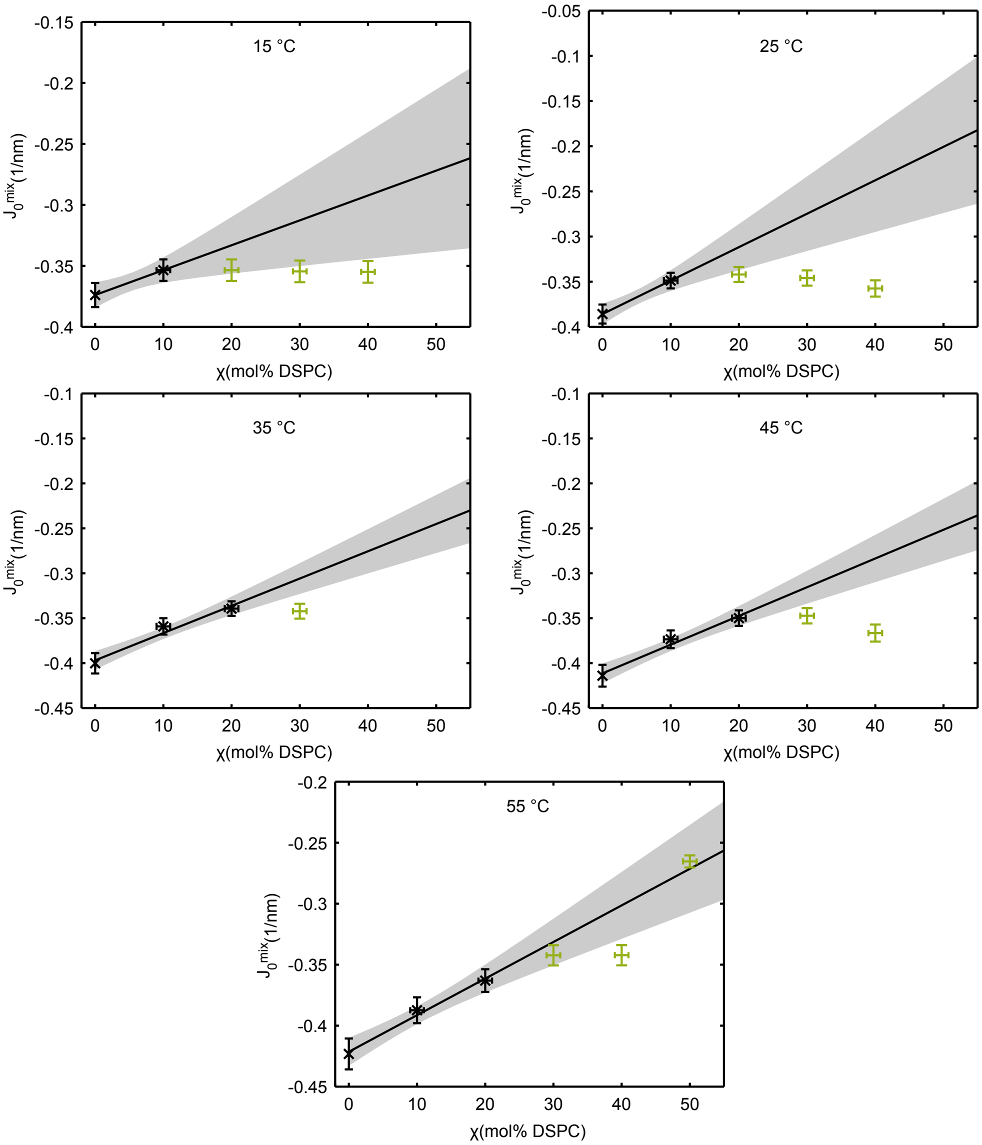


Figure S7: Determination of $J_0$ for DSPC.

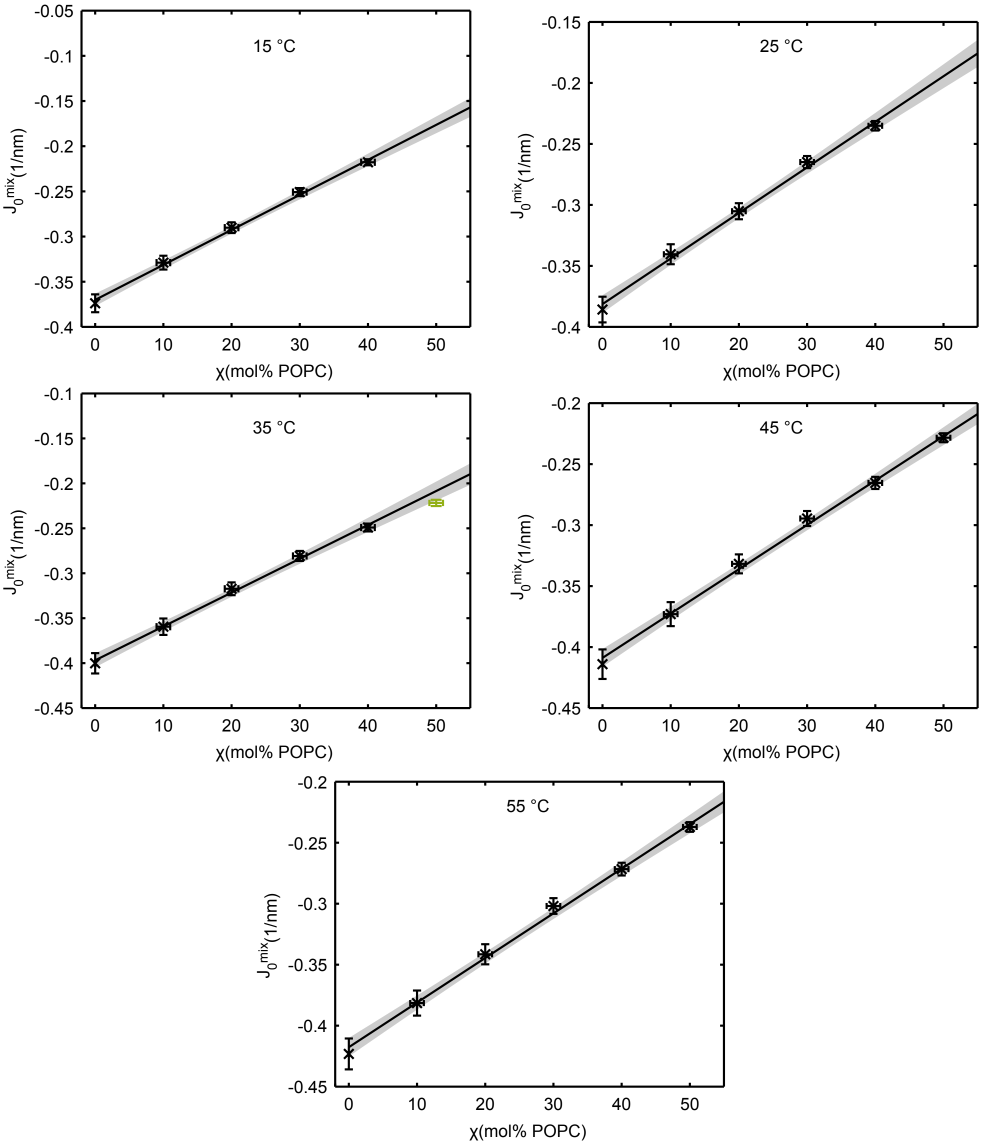


Figure S8: Determination of $J_0$ for POPC.

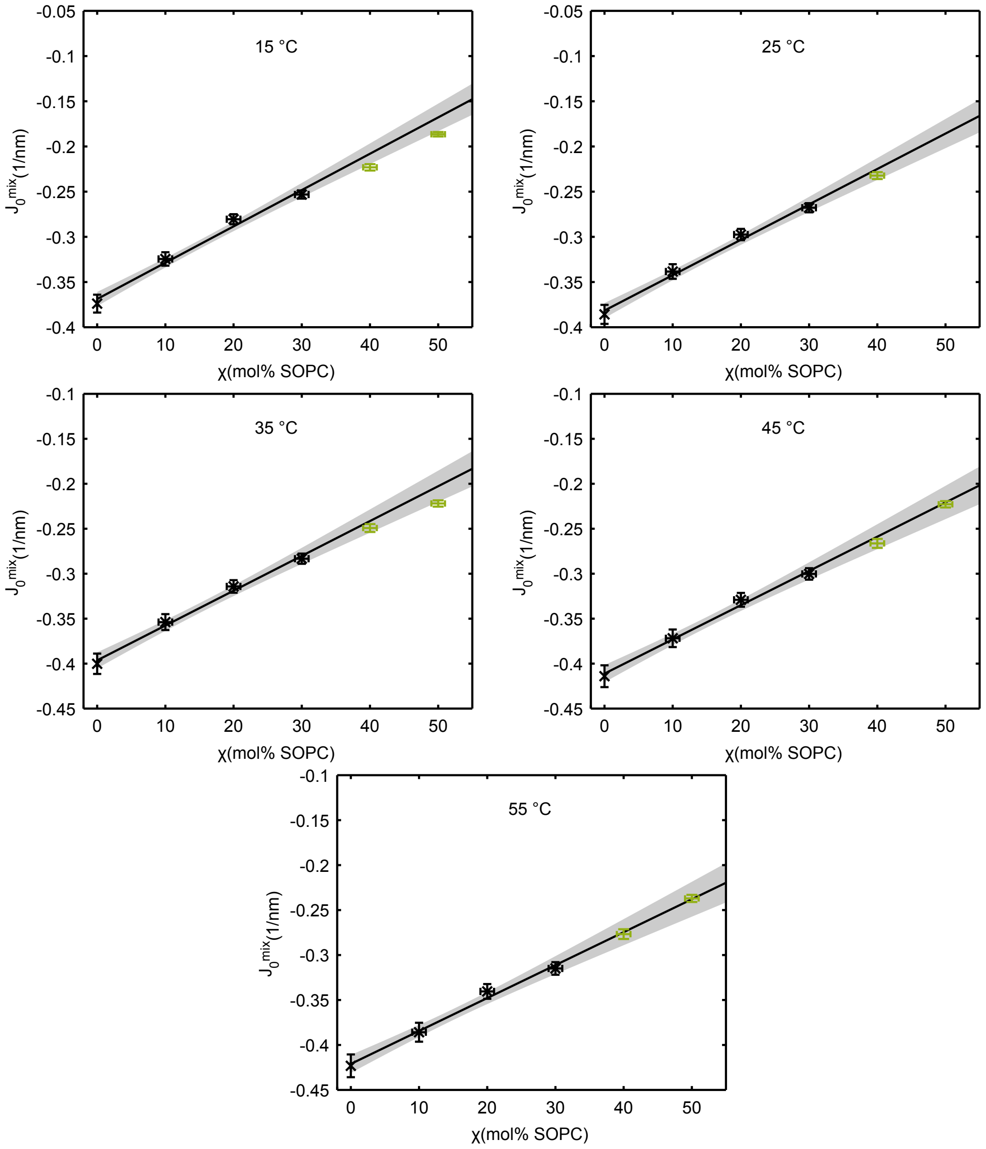


Figure S9: Determination of $J_0$ for SOPC.

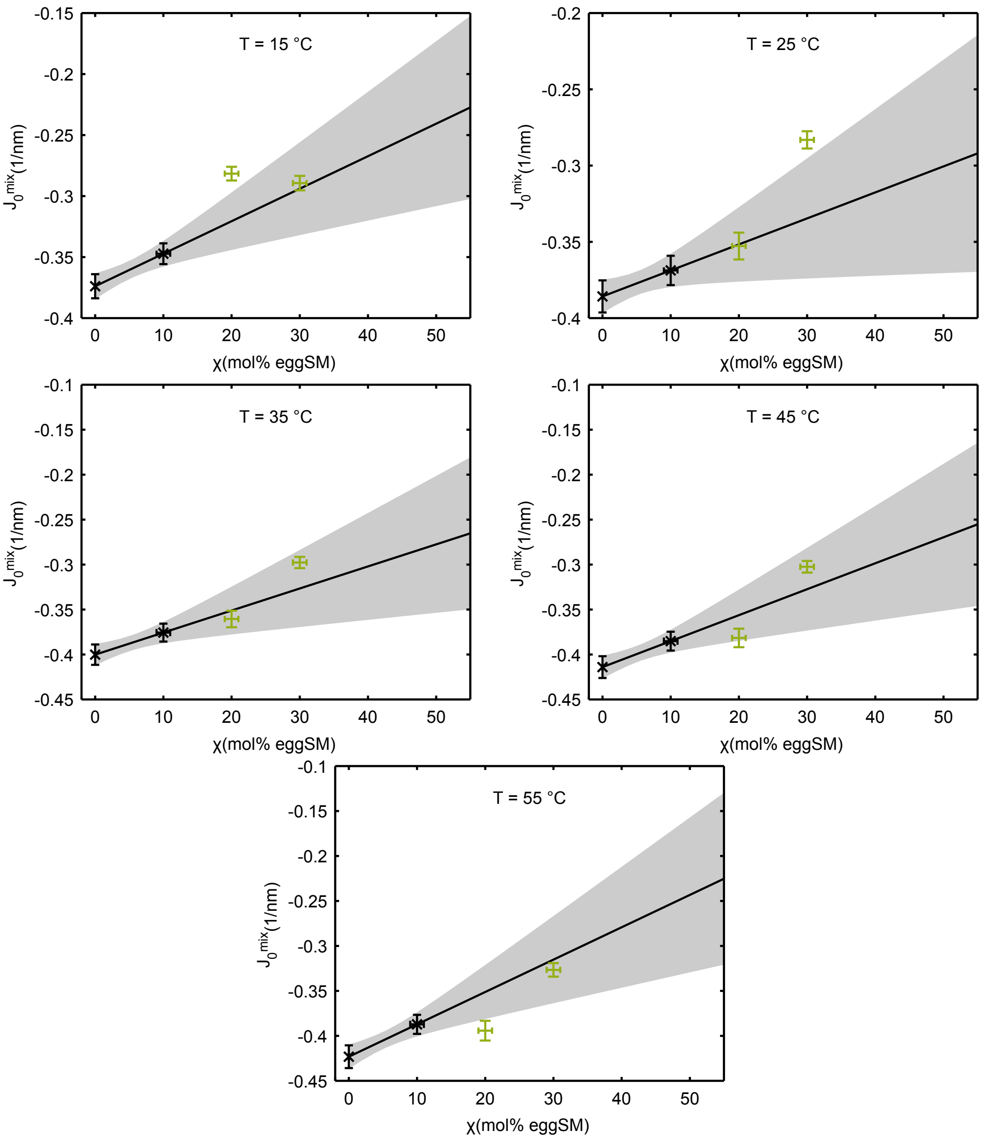


Figure S10: Determination of $J_0$ for eggSM.

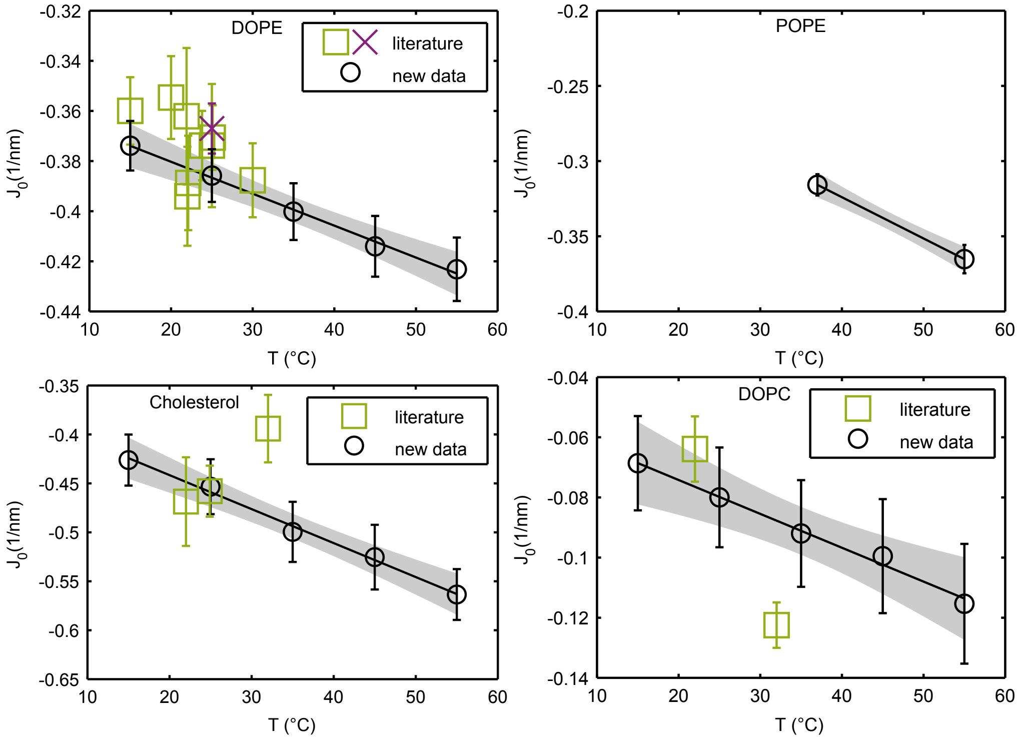


Figure S11: Temperature dependence of $J_0(T)$ compared with literature data.[16–24]

## S5 Temperature dependence of spontaneous curvature

Each lipid's spontaneous curvature $J_0(T)$ as a function of temperature $T$ is presented in Figs. S11–S12 (black circles) in comparison with literature data determined at the pivotal plane* (green squares) and the neutral plane (violet crosses). The black straight line is the result of the linear fit according to Eq. (2), while the gray band depicts its error via Eq. (3).

*Similar to Fig. 3, we rescaled reported values to $J_0 \sim J_{0p}(1+\beta)$, with $\beta = 0.065 \pm 0.035$ determined in[17].

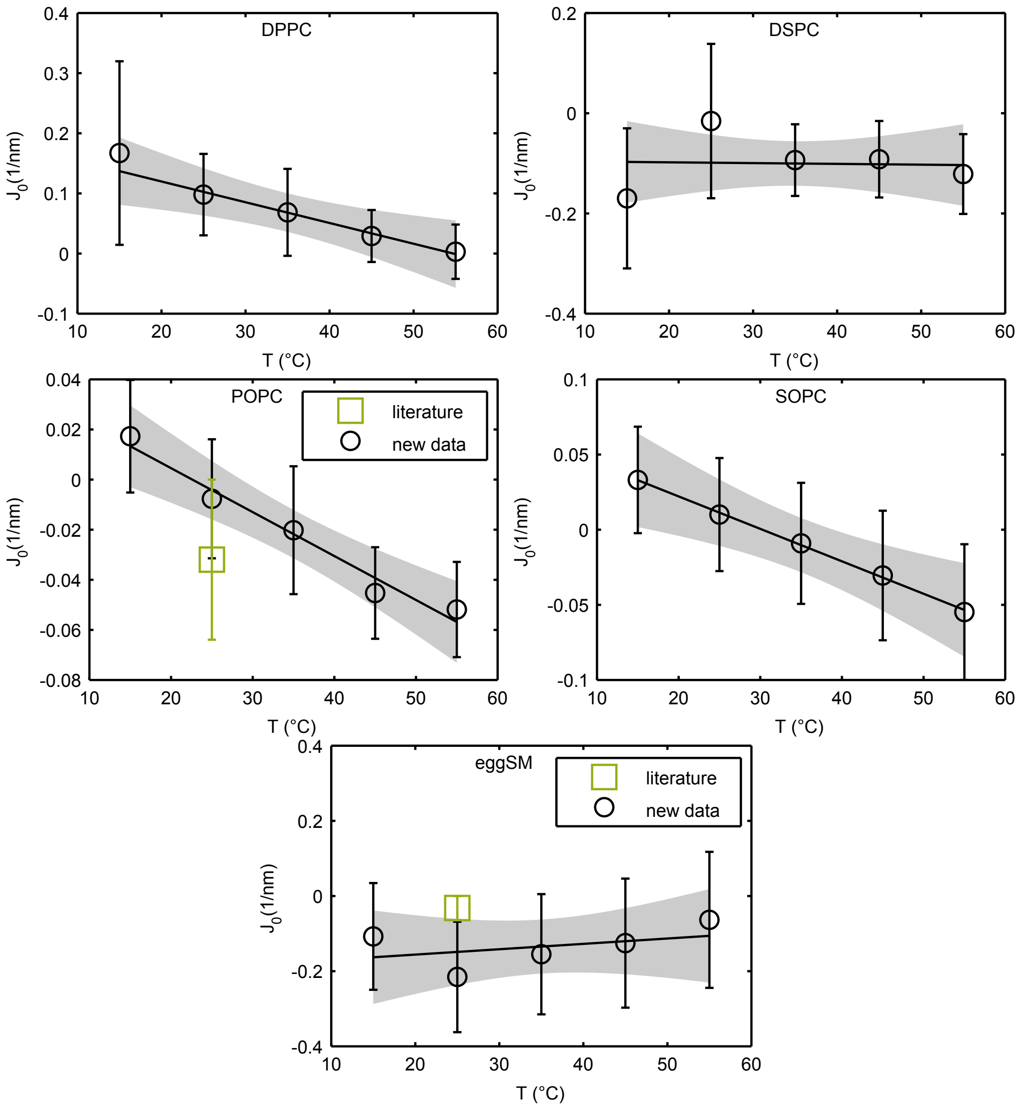


Figure S12: Temperature dependence of $J_0(T)$ compared with literature data.[22]

## References


[1] M. Rappolt, A. Hickel, F. Bringezu and K. Lohner, *Biophys. J.*, 2003, **84**, 3111–3122.

[2] B. E. Warren, *X-ray diffraction*, Addison-Wesley Pub. Co., Reading, Mass., 1969.

[3] D. C. Turner and S. M. Gruner, *Biochemistry*, 1992, **31**, 1340–1355.

[4] P. E. Harper, D. A. Mannock, R. N. Lewis, R. N. McElhaney and S. M. Gruner, *Biophys. J.*, 2001, **81**, 2693–2706.

[5] M. Rappolt, A. Hodzic, B. Sartori, M. Ollivon and P. Laggner, *Chem. Phys. Lipids*, 2008, **154**, 46–55.

[6] A. K. Smith and J. H. Freed, *J. Phys. Chem. B*, 2009, **113**, 3957–3971.

[7] F. A. Heberle, J. Wu, S. L. Goh, R. S. Petruzielo and G. W. Feigenson, *Biophys. J.*, 2010, **99**, 3309–3318.

[8] P. Uppamoochikkal, S. Tristram-Nagle and J. F. Nagle, *Langmuir*, 2010, **26**, 17363–17368.

[9] I. V. Ionova, V. A. Livshits and D. Marsh, *Biophys. J.*, 2012, **102**, 1856–1865.

[10] T. A. Pastva, *Master's thesis*, Naval Postgraduate School, Monterey, California, 1998.

[11] P. I. Kuzmin, S. A. Akimov, Y. A. Chizmadzhev, J. Zimmerberg and F. S. Cohen, *Biophys. J.*, 2005, **88**, 1120–1133.

[12] N. Kučerka, M.-P. Nieh and J. Katsaras, *Biochim. Biophys. Acta, Biomembr.*, 2011, **1808**, 2761–2771.

[13] A. I. Greenwood, S. Tristram-Nagle and J. F. Nagle, *Chem. Phys. Lipids*, 2006, **143**, 1–10.

[14] G. Khelashvili, B. Kollmitzer, P. Heftberger, G. Pabst and D. Harries, *J. Chem. Theory Comput.*, 2013.

[15] F. A. Heberle, R. S. Petruzielo, J. Pan, P. Drazba, N. Kučerka, R. F. Standaert, G. W. Feigenson and J. Katsaras, *J. Am. Chem. Soc.*, 2013, **135**, 6853–6859.

[16] R. P. Rand and N. L. Fuller, *Biophys. J.*, 1994, **66**, 2127–2138.

[17] S. Leikin, M. M. Kozlov, N. L. Fuller and R. P. Rand, *Biophys. J.*, 1996, **71**, 2623–2632.

[18] E. E. Kooijman, V. Chupin, N. L. Fuller, M. M. Kozlov, B. de Kruijff, K. N. J. Burger and R. P. Rand, *Biochemistry*, 2005, **44**, 2097–2102.

[19] N. Fuller, C. R. Benatti and R. P. Rand, *Biophys. J.*, 2003, **85**, 1667–1674.

[20] Z. Chen and R. P. Rand, *Biophys. J.*, 1997, **73**, 267–276.

[21] M. M. Kozlov, S. Leikin and R. P. Rand, *Biophys. J.*, 1994, **67**, 1603–1611.

[22] B. Boulgaropoulos, M. Rappolt, B. Sartori, H. Amenitsch and G. Pabst, *Biophys. J.*, 2012, **102**, 2031–2038.

[23] J. A. Szule, N. L. Fuller and R. P. Rand, *Biophys. J.*, 2002, **83**, 977–984.

[24] R. P. Rand, N. L. Fuller, S. M. Gruner and V. A. Parsegian, *Biochemistry*, 1990, **29**, 76–87.
